# Supplementary material for: Liquid-Like Interfaces Mediate Structural Phase Transitions in Lead Halide Perovskites
Source: arXiv:1907.13509 ancillary file (2019-07-31)
Supplement: Supplementary file 1 [file SupplementaryInformation-Bischak-Lai_2019-07-25.docx.pdf]

# Supplementary Materials

## Liquid-Like Interfaces Mediate Structural Phase Transitions in Lead Halide Perovskites

Connor G. Bischak<sup>1\*†</sup>, Minliang Lai<sup>1\*</sup>, Dylan Lu<sup>1</sup>, Zhaochuan Fan<sup>2</sup>, Philippe David<sup>2</sup>, Dengpan Dong<sup>8</sup>, Hong Chen<sup>1, 9</sup>, Ahmed S. Etman<sup>10,11#</sup>, Teng Lei<sup>1</sup>, Junliang Sun<sup>12</sup>, Michael Grünwald<sup>2</sup>, David T. Limmer<sup>1,3,5</sup>, Peidong Yang<sup>1,3,5,7,\*</sup>, Naomi S. Ginsberg<sup>1,3,4,5,6,\*</sup>

### Affiliations:

<sup>1</sup>Department of Chemistry, University of California, Berkeley, CA 94720.

<sup>2</sup>Department of Chemistry, University of Utah, Salt Lake City, Utah 84112.

<sup>3</sup>Materials Sciences Division, Lawrence Berkeley National Laboratory, Berkeley, CA 94720.

<sup>4</sup>Department of Physics, University of California, Berkeley, CA 94720.

<sup>5</sup>Kavli Energy NanoScience Institute, Berkeley, CA 94720.

<sup>6</sup>Molecular Biophysics and Integrative Bioimaging Division, Lawrence Berkeley National Laboratory, Berkeley, CA 94720.

<sup>7</sup>Department of Materials Science and Engineering, University of California, Berkeley, CA 94720

<sup>8</sup>Department of Materials Science and Engineering, University of Utah, Salt Lake City, Utah 84112.

<sup>9</sup>School of Environmental Science and Engineering, Southern University of Science and Technology, Shenzhen, Guangdong, China

<sup>10</sup>Department of Materials and Environmental Chemistry (MMK), Stockholm University, SE 106 91 Stockholm, Sweden.

<sup>11</sup>Department of Chemistry, Faculty of Science, Alexandria University, Ibrahimia, 21321 Alexandria, Egypt.

<sup>12</sup>College of Chemistry and Molecular Engineering, Peking University, Beijing 100871, China

\*These authors contributed equally to this work.

\*Corresponding authors. Email: nsginsberg@berkeley.edu , p\_yang@berkeley.edu

†Present Address: Department of Chemistry, University of Washington, Seattle, WA 98195.

#Present Address: Department of Physics, Chemistry and Biology (IFM), Linköping University, 581 83, Linköping, Sweden.

Correspondence to: nsginsberg@berkeley.edu, p\_yang@berkeley.edu

**This PDF file includes:**

Experimental Materials and Methods  
Molecular Dynamics Methods  
Ising Model Simulations of Nucleation and Early Growth  
Supplementary Figures S1 to S18  
Supplementary Tables S1 to S2  
Captions for Movies S1 to S4  
Supplementary References

**Other Supplementary Materials for this manuscript include the following:**

Movies S1 to S4

## Experimental Materials and Methods

### Low-temperature phase CsPbI<sub>x</sub>Br<sub>3-x</sub> nanowire synthesis

All of the chemicals were purchased from Sigma-Aldrich unless otherwise stated. 460mg PbI<sub>2</sub> (99.999%) was dissolved in 1 mL anhydrous dimethylformamide (DMF), stirred at 70 ° C overnight before further use. The PbI<sub>2</sub> solution was spin on O<sub>2</sub> plasma treated glass substrates at 3,000 rpm for 60 s, then annealed at 100 ° C for 15 min. The PbI<sub>2</sub> film was carefully dipped into a glass vial with a mixed solution of 0.4 mL 8 mg/ml CsI (99.999%)/methanol (anhydrous 99.8%), 1ml 8mg/CsBr (99.999%)/methanol (anhydrous 99.8%) and 0.8 ml methanol (anhydrous 99.8%). The PbI<sub>2</sub> side was facing up during the reaction. The reaction was carried at room temperature for 12 h with the glass vial capped tightly, then the substrate was taken out to wash in anhydrous isopropanol for 30 s. Then the sample was dried under 50 ° C for 5 min. The whole growth process was in a N<sub>2</sub> filled glovebox. The PL emission peak of the corresponding heating transformed high-T phase is the same as the CsPbBr<sub>2</sub>I composition in our previous report (1).

### Photoluminescence (PL) spectra

Photoluminescence measurements were performed by OBIS 375nm LX 50mW Laser (The intensity of the beam is 1 mW) with emission collected on a Nikon A1 microscope coupled to a multimode fiber coupled to a liquid-nitrogen-cooled Si CCD.

### X-ray diffraction (XRD)

The XRD pattern was acquired by using a Bruker AXS D8 Advance diffractometer equipped with a lynxeye detector, which used Cu K $\alpha$  radiation. GIWAXS data of the low-temperature to high-temperature transition were collected at SSRL beamline I11-3. The glass substrate with as-grown nanowires was heated in situ on a hot plate in a helium chamber.

### Selected area electron diffraction (SAED):

LT-CsPbIBr<sub>2</sub> nanowires were transferred by lightly pressing a TEM grid on a nanowire film. For HT-CsPbIBr<sub>2</sub> nanowires, LT-CsPbIBr<sub>2</sub> nanowires were transferred on a TEM grid first, then were heated through the phase transition process in a glovebox. The TEM images and SAED patterns

in **Figure S1** were acquired by using the FEI Titan microscope at the National Center for Electron Microscopy. All the measurements were performed at 300 kV.

#### Continuous rotation electron diffraction (cRED):

The dried film was scratched from the glass substrate and then coated on a copper grid with the carbon film (STEM150 Cu grids, Okenshoji) directly. The three-dimensional reciprocal lattice of both low-temperature and high-temperature phases were reconstructed from continuous rotation electron diffraction (c-RED) (2) data (**Figure S1**). The cRED was collected using the transmission electron microscope (TEM, JEOL JEM-2100-LaB<sub>6</sub>) operated at an accelerating voltage of 200 kV. The sample was cooled down to -178 °C using cryo-holder filled with liquid N<sub>2</sub>. A Gatan Orius camera was used for imaging and locating appropriate crystals for electron diffraction data collection. The cRED data were collected via continuous tilting of the goniometer in the angle range between  $\pm 30^\circ$ . A high-speed hybrid TimePix camera (Amsterdam Scientific Instrument) operated by SoPhy software was used for recording the cRED data. The data was processed using X-ray Detector Software (XDS) (3) and RED processing software (REDp) (4). Transmission electron microscopy (TEM) bright-field images and energy dispersive spectra were also collected on the same TEM.

#### Cathodoluminescence (CL) microscopy

Cathodoluminescence (CL) and secondary electron (SE) images were collected with a Zeiss Gemini SUPRA 55 S2 Scanning Electron Microscope (SEM) modified with a home-built CL detection setup and a home-built heater stage with custom ScopeFoundry Software (5). An aluminum parabolic reflector was positioned above the sample in order to couple a  $1.3\pi$  sr solid angle of emission into a photomultiplier tube (Hamamatsu, H7421-40) outside of the vacuum chamber. All CL images were acquired with 512 x 512 pixels, a scan rate of ~10 ms/line, a beam current of ~300 pA, and an accelerating voltage of 3.0 kV. The heater is comprised of a 0.32-inch diameter O<sub>2</sub> button heater (101275-29, HeatWave Labs) with a thermocouple temperature read-out placed adjacent to the sample on an identical Si substrate. For monitoring the phase transition upon heating, the temperature was ramped to an initial set point and then held constant (**Figure S4**). CL image acquisition was initiated at the initial set point and recorded until the phase transition was complete.

#### Analysis of nanowire perovskite phase propagation

Analysis of perovskite phase propagation was performed in Matlab R2017B and is summarized in **Figure S5**. CL image time series were first registered to account for lateral drift by first registering the SE image series and then applying the image registration to the corresponding CL dataset. Nanowires were then selected from the larger field of view, cropped, and reoriented. Overlapping nanowires and nanowires that moved during CL image series acquisition were not included in the analysis of phase propagation rates. Phase propagation rates were determined for individual nucleation events by measuring the movement of the 50% CL intensity point at the phase boundary along the length of the nanowire. The analysis was repeated for different temperature set points to generate the histogram data shown in **Figure 2A**. At temperatures higher than ~185 °C, propagation rates could not be determined because the rates exceeded the temporal resolution of our CL imaging.

#### Analysis of perovskite nucleation events

Analysis of nucleation events was performed in ImageJ 1.51w and Matlab R2017B. The nucleation analysis is summarized in **Figure S11**. CL image time series were registered as described above. Initial nucleation event times were determined by identifying pixels with an intensity value 1.5x the nanowire background CL. Later nucleation times were identified as the time that nuclei reached ~250 nm across (similar to the width of the nanowires). Plots of the number of nucleation events versus time were fit with the Johnson-Mehl-Avrami-Kolmogorov equation (**Figure S12**):

$$x(t) = 1 - \exp(-kt^n)$$

where  $x(t)$  is the number of nucleation events in time,  $k$  is the convolved rate of nucleation and growth to reach the size threshold, and  $n$  is related to the geometry of the transformation.

#### Measurement and analysis of individual nucleation events

To visualize the growth of individual nuclei, CL time series were acquired at a smaller field-of-view of 5 x 5 μm. Individual nuclei were cropped and plotted as a time series. Circularity analysis

was performed in ImageJ 1.51w by thresholding the intensity of the nuclei and measuring the circularity with the following equation:

$$c = 4\pi\left(\frac{A}{P^2}\right)$$

where  $A$  is the area of the nucleus and  $P$  is the perimeter.

## Molecular Dynamics Methods

### Material composition: CsPbBr<sub>3</sub> vs. CsPbIBr<sub>2</sub>

In our simulations, we use a force field for CsPbBr<sub>3</sub> to study phase transitions of experimental CsPbIBr<sub>2</sub> nanowires. This choice was made because a reliable force field for the four-component mixed halide system is considerably more difficult to obtain than for CsPbBr<sub>3</sub>. The two materials have somewhat different phase diagrams. In particular, the non-perovskite LT-CsPbBr<sub>3</sub> phase is not thermodynamically stable for CsPbBr<sub>3</sub>, but it is metastable and not significantly less stable than for CsPbIBr<sub>2</sub> at comparable temperatures (1). Furthermore, vacancy formation energies and activation barriers for vacancy hopping are very similar for different halides and independent of composition (6). Based on data given in Ref. 6, we estimate that the energy scales for defect diffusion and rearrangement in CsPbBr<sub>3</sub> and CsPbIBr<sub>2</sub> differ by no more than 5-10%. Since the growth mechanism observed in our simulations involves similar microscopic rearrangements, we expect that differences in the activation energy for growth are of the same magnitude, well within the uncertainty of our calculations.

### Parameterization of CsPbBr<sub>3</sub> force field

We use pairwise additive, radially symmetric interactions to model CsPbBr<sub>3</sub> crystals. The pair potentials consist of short-range repulsive and attractive dispersion forces, as well as Coulomb interactions. Specifically, ions of type  $i$  and  $j$  interact via

$$u_{ij}(r) = \frac{q_i q_j}{4\pi\epsilon_0 r} + 4\epsilon_{ij} \left[ \left(\frac{\sigma_{ij}}{r}\right)^{12} - \left(\frac{\sigma_{ij}}{r}\right)^6 \right].$$

Similar models have been successfully used in the past to model other ionic semiconductor solids (7). Lennard-Jones parameters for interactions between ions of the same type ( $\varepsilon_{\text{Cs}}$ ,  $\varepsilon_{\text{Pb}}$ ,  $\varepsilon_{\text{Br}}$ ,  $\sigma_{\text{Cs}}$ ,  $\sigma_{\text{Pb}}$ , and  $\sigma_{\text{Br}}$ ) were determined by fitting to lattice constants, elastic properties, and energy differences between different crystal structures, as described below; standard combining rules,  $\varepsilon_{ij} = \sqrt{\varepsilon_i \varepsilon_j}$  and  $\sigma_{ij} = (\sigma_i + \sigma_j)/2$ , were used to determine cross-interactions. For the ionic charges  $q$ , we use partial charges determined by Bader charge analysis (8) in the cubic perovskite structure (HT-CsPbBr<sub>3</sub> phase), as described below. Final force field parameters are listed in **Table S1**; the pair potentials are plotted in **Figure S7**.

The data set used for fitting included lattice constants, elastic properties, and energy differences of five crystal structures of CsPbBr<sub>3</sub>. These data were obtained from density functional theory (DFT) calculations carried out with the Vienna Ab-initio Simulation Package (VASP) (9) with the projector augmented wave (PAW) method (10). We initially compared data obtained with three different density functionals, including GGA-PBE (11), PBEsol (12), and SCAN (13). A cutoff energy of 600 eV and Monkhorst-Pack k-meshes with a minimum spacing of 0.2 Å<sup>-1</sup> were used in all calculations. We considered five different polymorphs of CsPbBr<sub>3</sub>, including four perovskite structures and the non-perovskite LT-CsPbBr<sub>3</sub> phase. The four perovskite structures include the well-known cubic (space group #221) and orthorhombic (space group #62) phases, as well as two tetragonal (space group #127 and #140) structures and the non-perovskite orthorhombic LT-CsPbBr<sub>3</sub> phase (space group #62). All structures were fully relaxed till forces were converged to within 5 meV/Å. All DFT results are listed in **Table S2**. While PBEsol and SCAN produced comparable values, lattice parameters obtained with PBEsol overall provided the best match with known experimental values. We therefore chose to use PBEsol data as reference for lattice constants and elastic properties. (Note that experimental values were obtained at finite temperature, while DFT values are ground state (0 K) energies.) However, among the three DFT methods only PBE yielded the correct energetic order of crystal structures (*i.e.*,  $E_{\text{HT-ort}} < E_{\text{HT-tet}} < E_{\text{HT-cub}}$ ;  $E_{\text{HT-ort}} < E_{\text{LT}}$ ) (14). We therefore chose energy differences obtained with PBE as the reference for our force field parameterization.

We used a Monte Carlo simulated annealing (MCSA) method (15, 16) to fit the six remaining force field parameters ( $\varepsilon_{\text{Cs}}$ ,  $\varepsilon_{\text{Pb}}$ ,  $\varepsilon_{\text{Br}}$ ,  $\sigma_{\text{Cs}}$ ,  $\sigma_{\text{Pb}}$ , and  $\sigma_{\text{Br}}$ ) to the DFT data. Compared to more

straightforward methods (*e.g.*, gradient descent), the MCSA method more efficiently samples high-dimensional parameter spaces and provides a means of escaping local minima in the fitness landscape, defined via

$$f = \sum_{i=1}^N \sqrt{w_i (A_i^o - A_i^c)^2}.$$

Here,  $N$  is the total number of fitted quantities,  $A_i^c$  and  $A_i^o$  are the force field and reference values of the  $i$ th quantity, respectively, and  $w_i$  is the fitting weight assigned to that quantity. All properties of the force field model (lattice and elastic constants, bulk modulus, and energy differences) were calculated with GULP (17). As fitting weights for energy differences, lattice parameters, fractional coordinates, bulk modulus, and elastic constants, we used  $10000 \text{ (eV/f.u.)}^{-2}$ ,  $1000 \text{ \AA}^{-2}$ ,  $1000 \text{ \AA}^{-2}$ ,  $10 \text{ GPa}^{-2}$ , and  $1 \text{ GPa}^{-2}$ , respectively. Starting from a given set of parameters  $s_o$ , in an elementary MC step of the fitting procedure, a single parameter was randomly selected and appropriately modified to produce a trial parameter set  $s_t$ . The trial parameter set was accepted or rejected according to the standard Metropolis criterion,  $p(s_o \rightarrow s_t) = \min[1, e^{(f_t - f_o)/T}]$ , where  $f_t$  and  $f_o$  are the fitness of the trial and original parameter sets, respectively, and  $T$  is a fictitious temperature-like quantity.  $T$  was initially set to 1.0 and was gradually reduced by multiplication with a factor of 0.997 every 50 MC steps. In each MCSA run,  $10^5$  MC steps were performed, resulting in a final value of  $T = 0.00246$ . 24 independent MCSA runs were performed from different initial parameter sets to efficiently scan the parameter space. **Figure S6** shows the evolution of  $f$  for all 24 MCSA runs; the red line indicates the run which yielded the best parameters. The final parameter set is provided in **Table S1** and the quantities used for fitting are compared to their reference values in **Table S2**.

### MD simulations

MD simulations were carried out using the LAMMPS simulation package (18). All simulations were performed in the NPT ensemble at zero pressure and a time step of 2 fs. Temperature and pressure were controlled by a Nose-Hoover thermostat and barostat, respectively, as implemented in LAMMPS. We simulated different interfaces between the LT-CsPbBr<sub>3</sub> and HT-CsPbBr<sub>3</sub> phases, including (100)<sub>HT</sub>/(100)<sub>LT</sub>, (110)<sub>HT</sub>/(100)<sub>LT</sub>, (110)<sub>HT</sub>/(010)<sub>LT</sub>, and (110)<sub>HT</sub>/(001)<sub>LT</sub>. Systems were first equilibrated at a temperature of 300 K for 2 ns, then the temperature was increased from 300 K to the target temperature (500, 520, or 540 K) in another 2 ns simulation. After equilibration,

long simulation runs (1-2  $\mu$ s) were performed at each temperature to observe the propagation of the boundary between the LT-CsPbBr<sub>3</sub> and HT-CsPbBr<sub>3</sub> phases and to measure transition rates. We performed 3-5 independent simulations of each system and temperature.

### Distinguishing HT-CsPbBr<sub>3</sub> and LT-CsPbBr<sub>3</sub> phases

We distinguish HT-CsPbBr<sub>3</sub> and LT-CsPbBr<sub>3</sub> phases based on different coordination environments of Pb ions in the two structures. Specifically, we used the number  $n$  of Br ions within a distance of 5.4 Å around a given Pb as an order parameter. As shown in **Figure S8**, while  $n = 6$  in the HT-CsPbBr<sub>3</sub> phase (corresponding to the coordination octahedron around a given Pb),  $n \approx 9$  in the LT-CsPbBr<sub>3</sub> phase, due to the fact that Br octahedra share edges in this structure. We thus characterize all Pb ions with  $n \leq 6$  as belonging to the HT-CsPbBr<sub>3</sub> phase and use the fraction of HT-CsPbBr<sub>3</sub> phase Pb ions as a proxy for the fraction of HT-CsPbBr<sub>3</sub> phase present in the simulation. **Figure S9** and **Figure S10** show the time evolution of the fraction of HT-CsPbBr<sub>3</sub> phase at different temperatures for two different interface configurations. We calculate the rate of interface propagation  $v$  from the slopes  $k$  of linear fits to these data via  $v = Lk/2$ , where  $L$  is the length of the simulation box side perpendicular to the HT-LT interface and the factor of 2 is included to account for the presence of two interfaces in the simulation box. In some simulations, we observed an initial stage of abnormally fast growth of the HT-CsPbBr<sub>3</sub> phase (see, for instance, the trajectory at 540 K in **Figure S9**), which we attribute to the relaxation of the initial configuration. To ensure that propagation rates calculated from our simulations are representative of a steady-state growth regime, we excluded the initial 200 ns from the analysis of all trajectories.

## Ising Model Simulations of Nucleation and Early Growth

In order to understand the relative importance of geometric, thermodynamic and kinetic factors in the nucleation and growth of the perovskite phase in the nanowires, we have simulated a simple Ising model with anisotropic energetics. Specifically, we have studied a Hamiltonian of the form

$$H = - \sum_{\langle ij \rangle} J_{ij} s_i s_j - \sum_i h_i s_i$$

where  $s_i = \pm 1$  are spin variables that represent the perovskite and non-perovskite phases,  $J_{ij}$  are pair interactions equal to  $J_x$  and  $J_y$  along the long and short axes of the lattice respectively, and  $h_i$  are local fields that are equal to  $h_b$  in the bulk of the lattice, and  $h_x$  and  $h_y$  on the exposed long and short surfaces. The calculations are done on a 2d square lattice, and we consider interactions between only nearest neighbor spins.

We study the model at  $Tk_B/J_x = 1.2$ , where  $k_B$  is Boltzmann's constant, which is well below the critical point and set  $h_b = -0.15$  so that spin up is metastable with respect to spin down. To study nucleation, which is a rare event, we compute the free energy to grow a cluster of size  $N_c$  down spins in a bulk lattice or in the presence of an extended interface, where the cluster is defined as that set of spins sharing a nearest neighbor of common spin state. We do this using umbrella sampling and Metropolis Monte Carlo with single spin flip moves (19). Previous studies have shown that for the Ising model, while classical nucleation theory is not able to quantitatively describe the nucleation kinetics of phase transformations, the size of the largest cluster is a good reaction coordinate for these kinetics (20). To sample these fluctuations, we add a potential of the form

$$U = \frac{k}{2} (N_c - N'_c)^2$$

where  $k$  is the spring constant restricting fluctuations which we take to be  $0.02 J_x$  and  $N'_c$  is the minimum of the potential, which we take to span 0-200 in steps of 10. We use MBAR to combine data from each window into the free energies in **Figure S15** for a variety of ratios  $J_y/J_x$ . In order

to match the relative nucleation rate found experimentally for the end to side nucleation we find that we must use  $h_x = -0.2$  and  $h_y = -0.15$  and that the relative nucleation rates are insensitive to  $J_y/J_x$ . though the absolute barrier changes.

In addition to computing nucleation rates from the nucleation barrier heights, we have computed the interface motilities as a function of  $J_y/J_x$ . Specifically, beginning in a nanowire of equal proportions of spin up and spin down, under the same conditions as those used in the calculation of the nucleation barrier height, we compute the mean time to convert the lattice into 90% spin down. The results of these calculations are shown in **Figure S15**. We find that choosing  $J_y/J_x = 1.5$  is sufficient to explain the factor of 3 growth rate difference measured experimentally. The distribution of first passage times and example trajectories shown in **Figure 3** of the main text are computed using these optimized conditions with a stopping point equal to  $1.1 N_c^*$ , where  $N_c^*$  is the critical cluster size determined by the maximum of the free energy function. In order to compare to experiments we associate a single Ising lattice site to a length scale of 2 nm and assign a single MC sweep to a timescale of 0.1 s. These scales are set in order to match the growth velocity and mean nucleation time at the end of the nanowire.

## Supplementary Figures

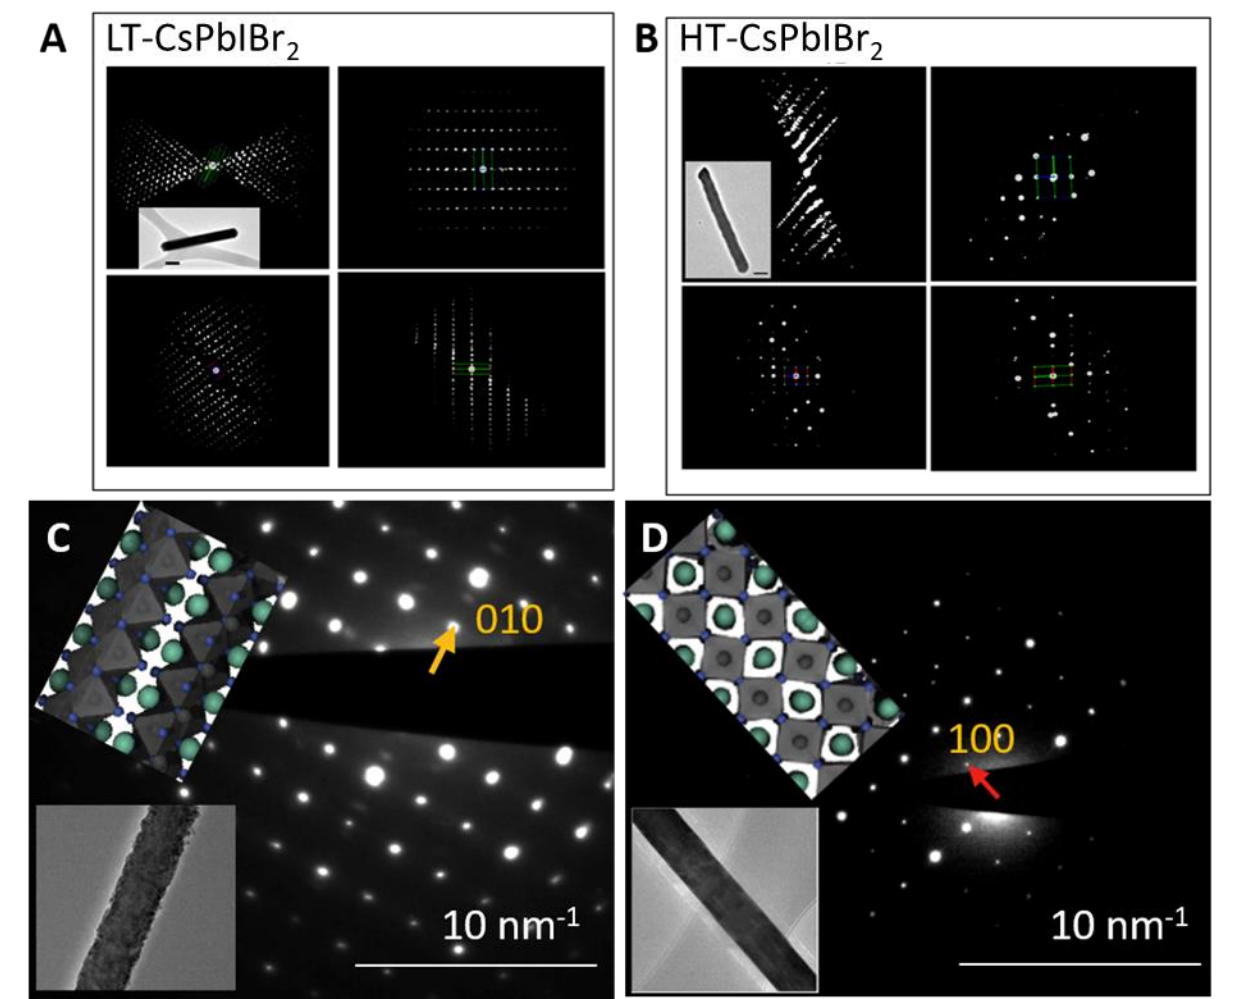

**Fig. S1. 3D reciprocal lattice of both phases reconstructed from the c-RED data and transmission electron microscopy single area electron diffraction (SAED).** (A) 3D reciprocal lattice of LT-CsPbIBr<sub>2</sub> showing that the octahedral chains are oriented along the length of the wire. (B) 3D reciprocal lattice of HT-CsPbIBr<sub>2</sub> after the phase transition is completed. (C,D) 2D projections of LT-CsPbIBr<sub>2</sub> and HT-CsPbIBr<sub>2</sub> nanowire diffraction, respectively, used in conjunction with c-RED data to determine the lead-halide octahedral packing direction along the nanowires. Altogether these data enable determination of the crystallographic configurations on either side of the interphase boundary.

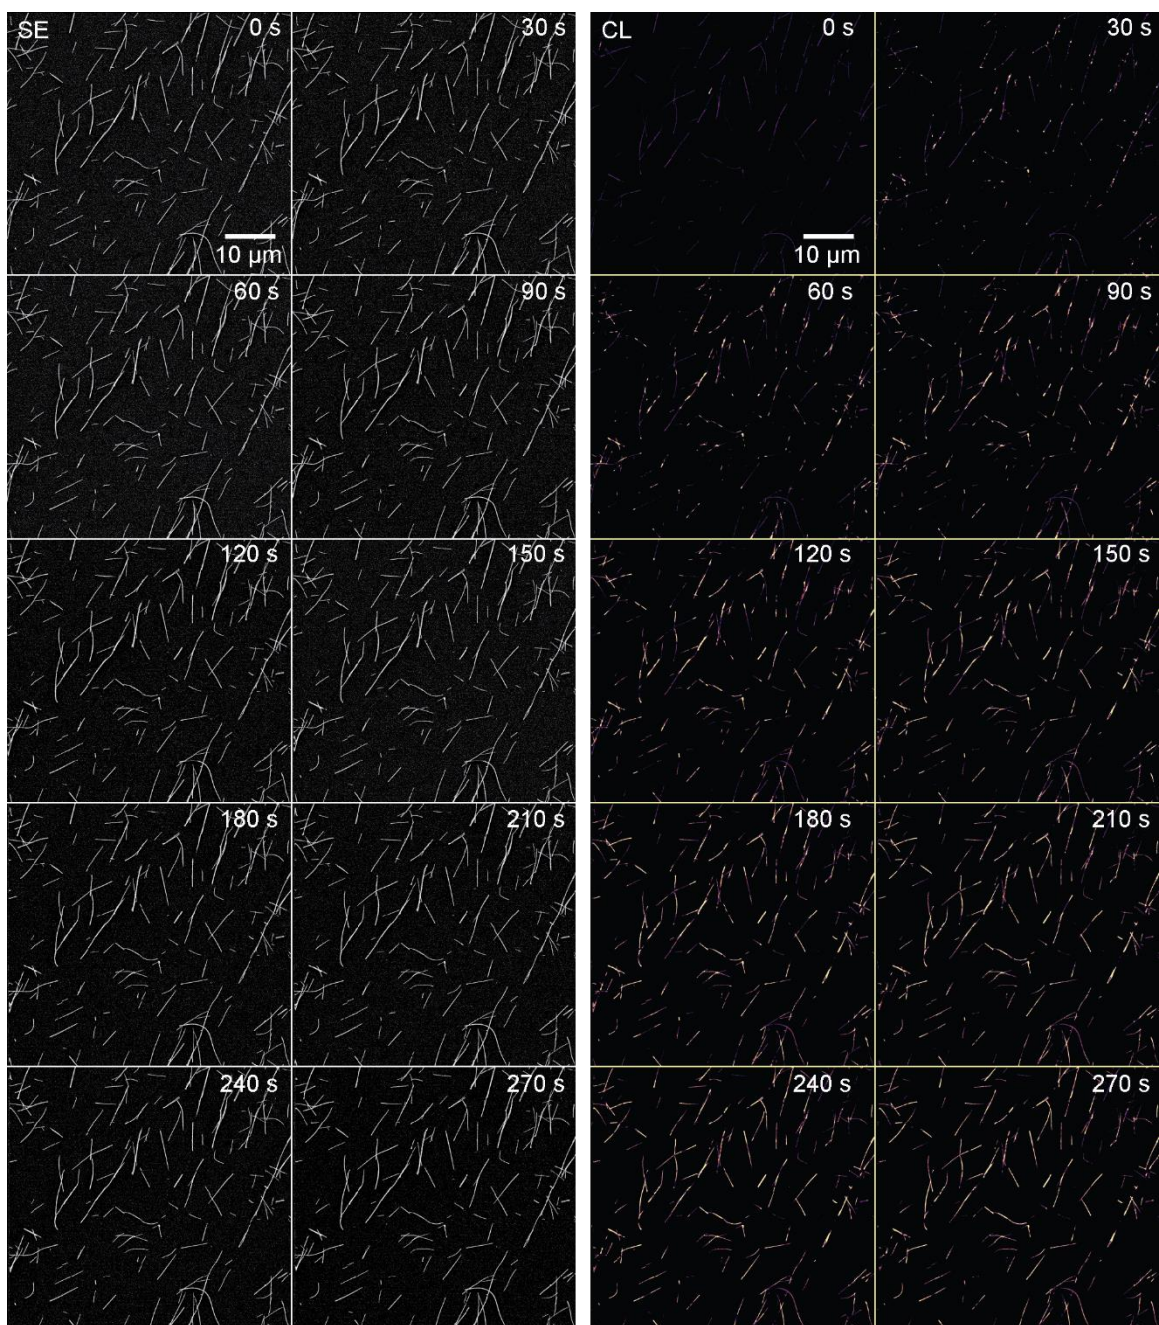

**Fig. S2. Time series of a larger field-of-view of CsPbIBr<sub>2</sub> nanowires undergoing the structural phase transition.** SE and CL time series of the same field-of-view as shown in **Figure 1D-F** and **Movie S1** showing nucleation and growth in > 100 nanowires simultaneously.

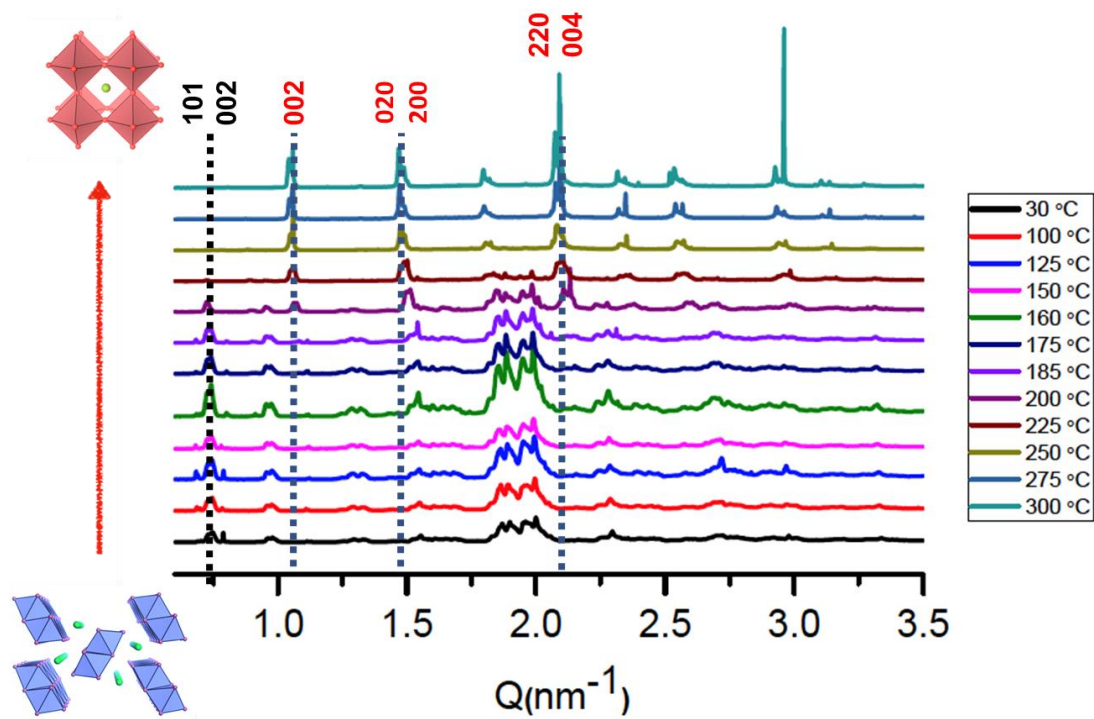

**Fig. S3.** *In situ* X-ray diffraction (XRD) of the LT-CsPbIBr<sub>2</sub> to HT-CsPbIBr<sub>2</sub> phase transition.

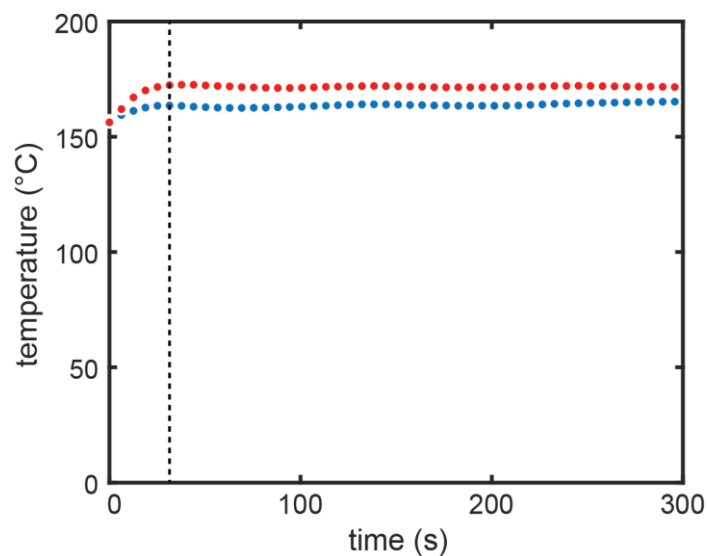

**Fig. S4. Example of temperature traces while acquiring SE and CL data to monitor the phase transition kinetics.** CL and SE images are recorded starting at 0 s. The dotted line represents when the temperature plateaus and phase front propagation rates are first recorded. The temperature was measured from a thermocouple on an Si substrate adjacent to the sample substrate (< 5 mm from the sample).

1) Align CL image time series based on SE image time series

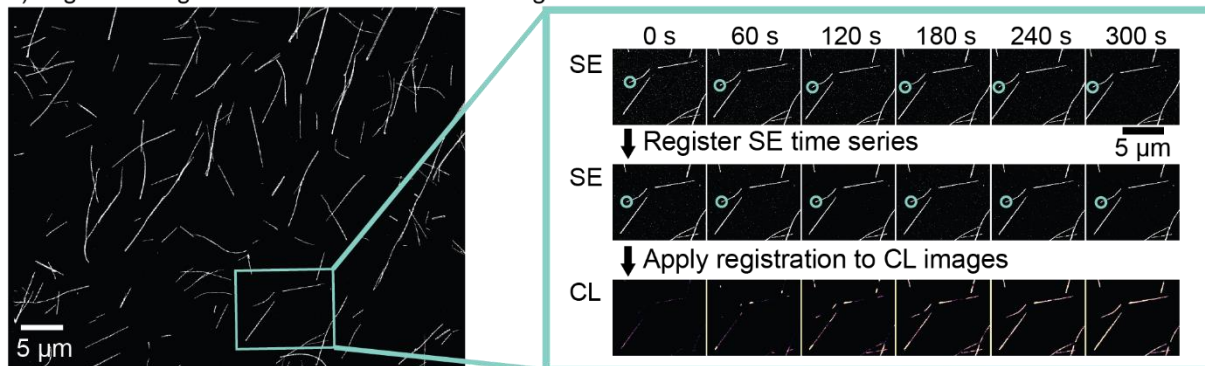

2) Select nanowire from the field-of-view, crop, and rotate

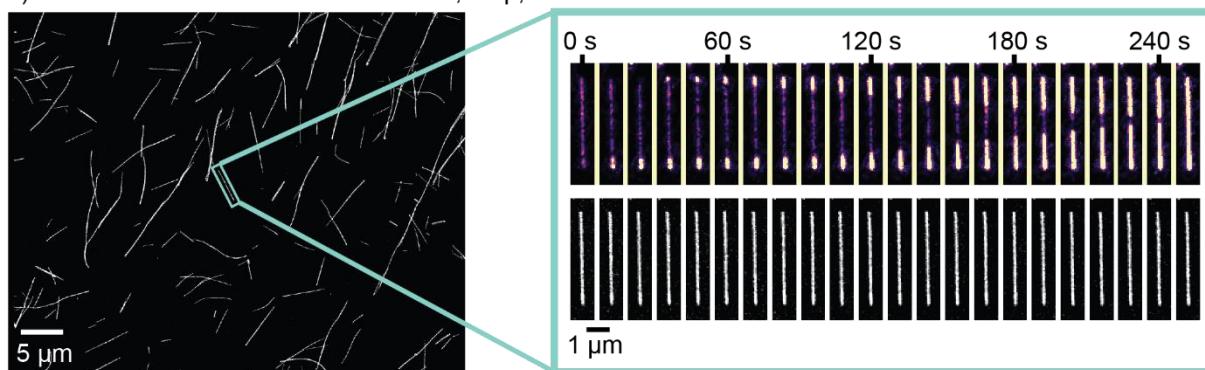

3) Track 50% CL intensity contour in time and find rate of propagation

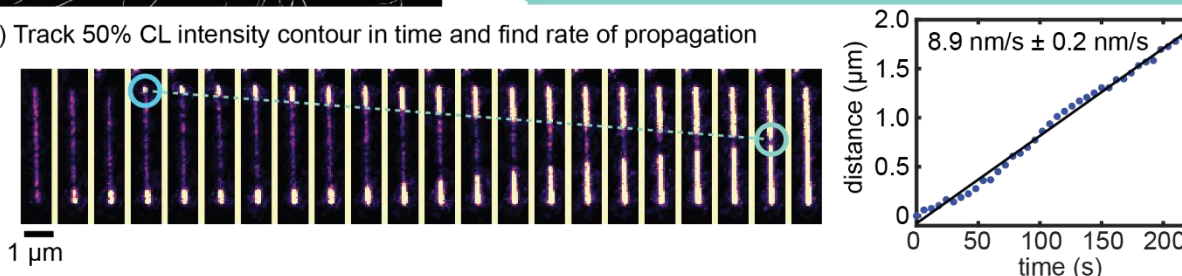

4) Repeat for other isolated wires in the field-of-view and for other fields-of-view at different temperatures

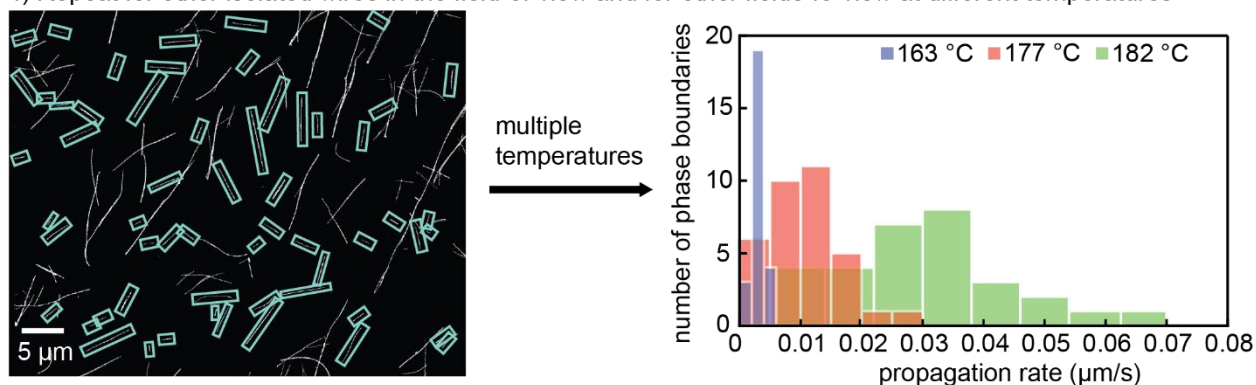

**Fig. S5. Workflow for analyzing nanowire phase propagation rates.** Large field-of-view SE and CL movies are aligned. Isolated wires are selected, cropped, and rotated. Propagation rates are measured based on the position of the 50% intensity contour. The process is repeated for many wires at different temperature to generate the histograms and Arrhenius plot shown in **Figure 2**.

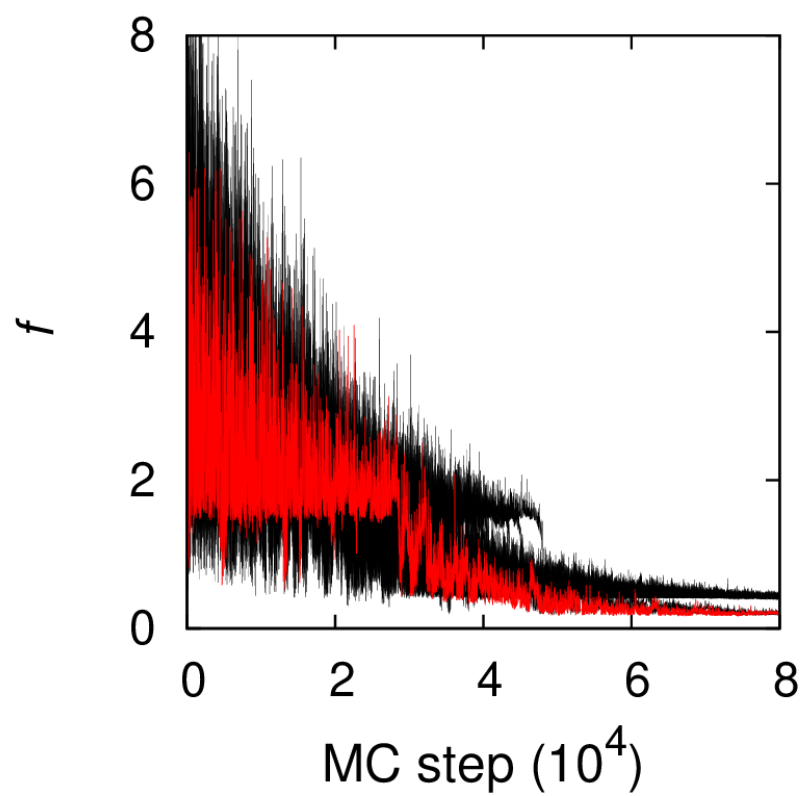

**Figure S6.** Evolution of the fitness function  $f$  during 24 MCSA runs. The MCSA run with the best parameter set is shown in red.

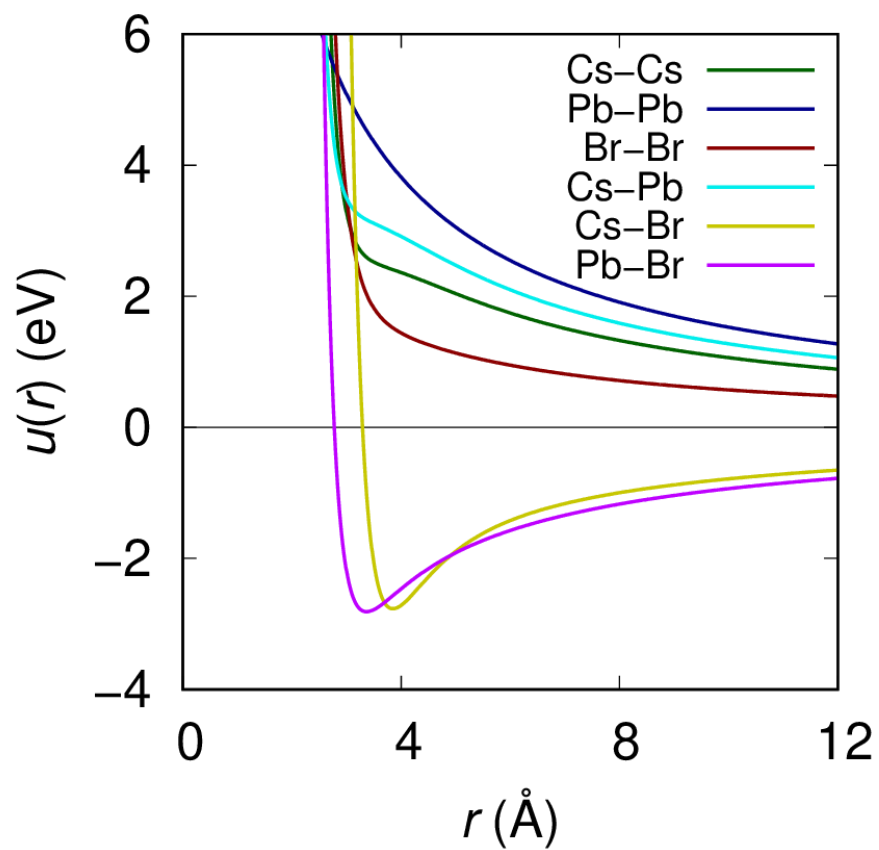

**Figure S7.** Plots of interaction potentials for all pairs of ion types.

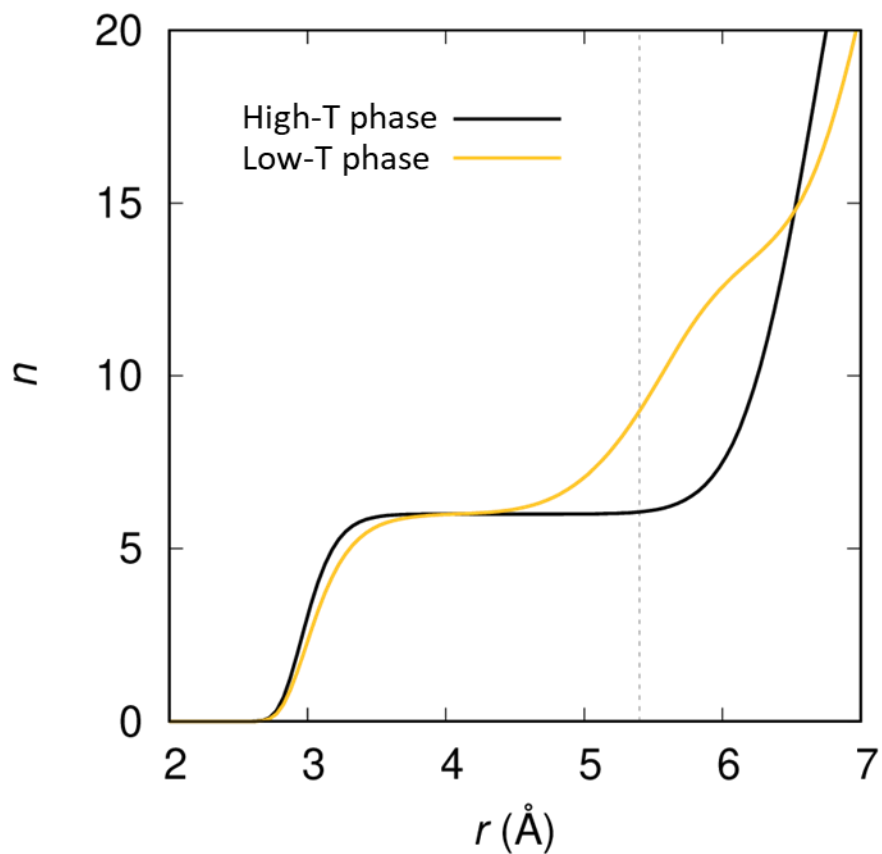

**Figure S8.** Average number  $n$  of Br ions within a distance  $r$  of a central Pb ion, for the high-T and low-T phases at 500 K. The vertical dashed line indicates the distance (5.4 Å) used to define the order parameter that distinguishes the LT-CsPbBr<sub>3</sub> and HT-CsPbBr<sub>3</sub> phases.

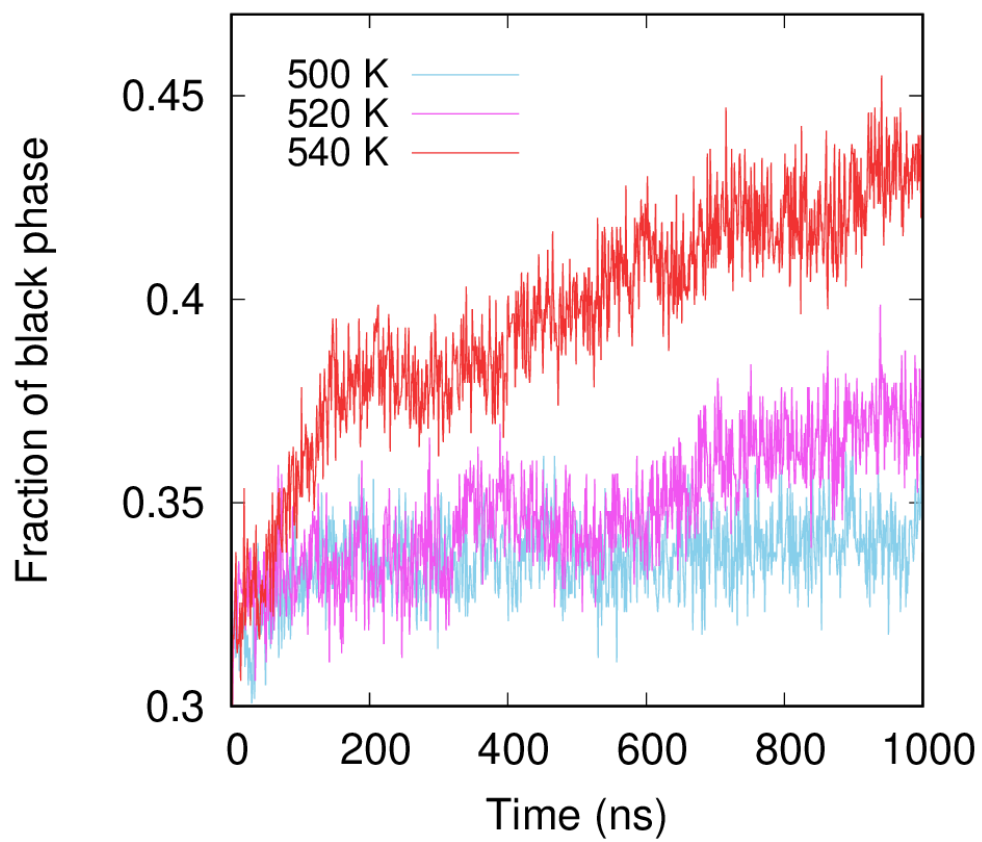

**Figure S9.** Time evolution of the fraction of HT-CsPbBr<sub>3</sub> phase in the HT(100)-LT(100) nanowire at three different temperatures.

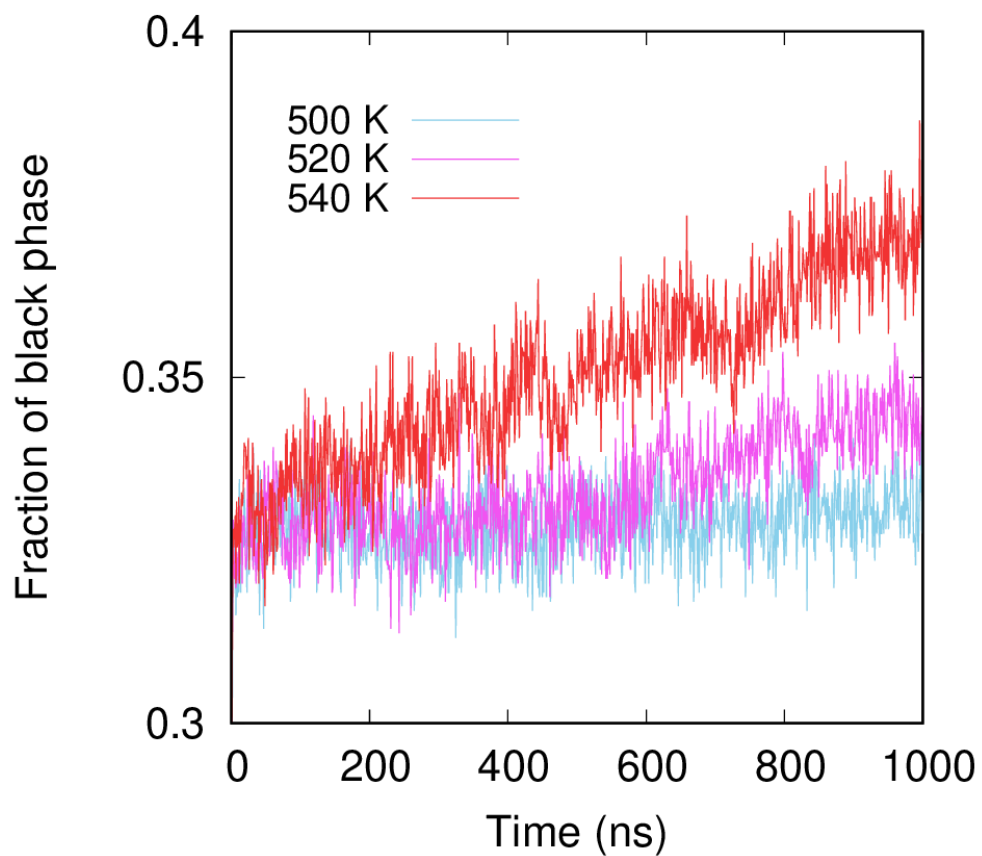

**Figure S10.** Time evolution of the fraction of HT-CsPbBr<sub>3</sub> phase in the HT(110)-LT(100) nanowire at three different temperatures.

1) Select areas where end and side nucleation events occur

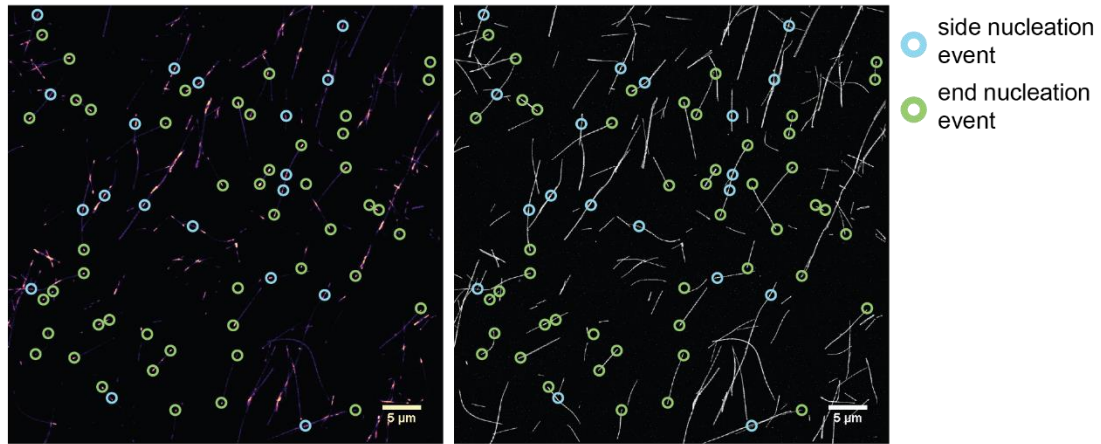

2) Find threshold for initial nucleation based on single pixel intensity above background (~50 nm) and later growth size (~250 nm)

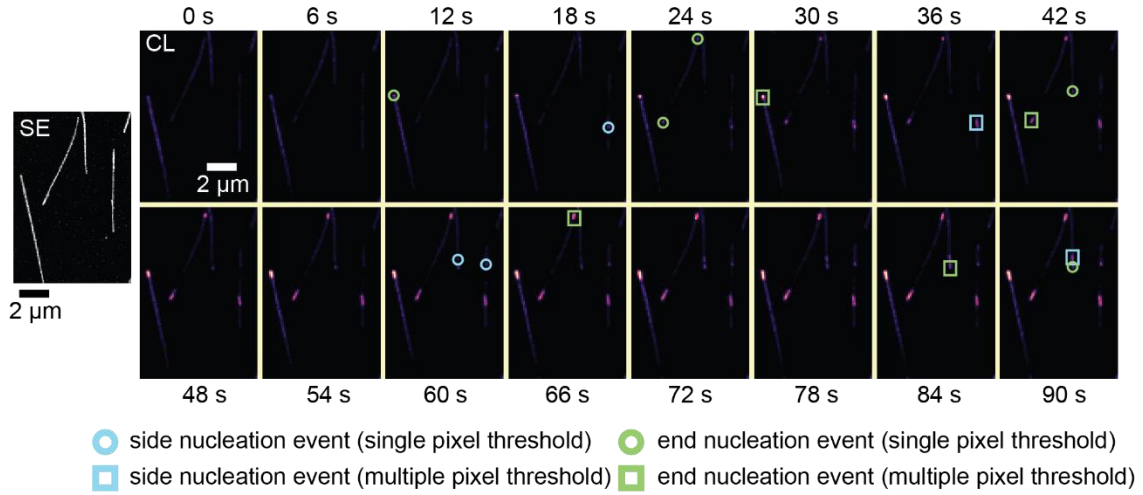

3) Repeat for all nucleation events in the field-of-view to generate histograms of end vs. side nucleation

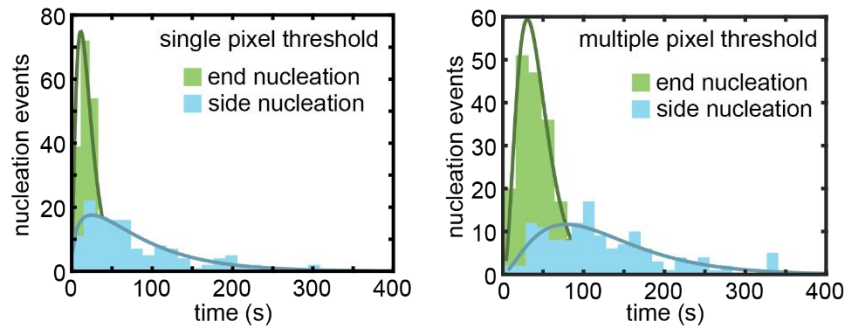

**Fig. S11. Workflow for analyzing nanowire nucleation events.** After registering the SE and CL images, nanowire end and side nucleation events are selected. Times of nucleation are recorded by taking the time that a single pixel intensity reaches a threshold higher than the background intensity. A multiple pixel threshold is also imposed to record later nucleation plus growth times (5 x 5 pixels above the background). After these data are recorded for a large field-of-view, histograms of the nucleation times are constructed.

## Initial nucleation

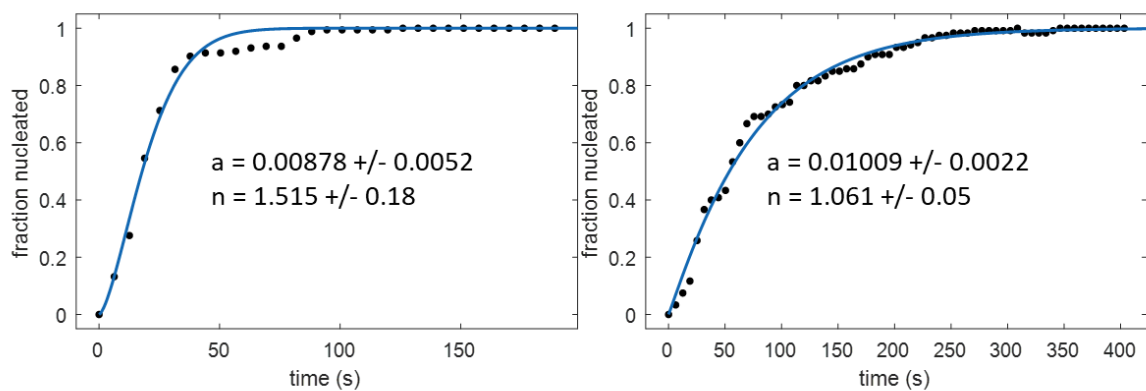

## Growth to wire width

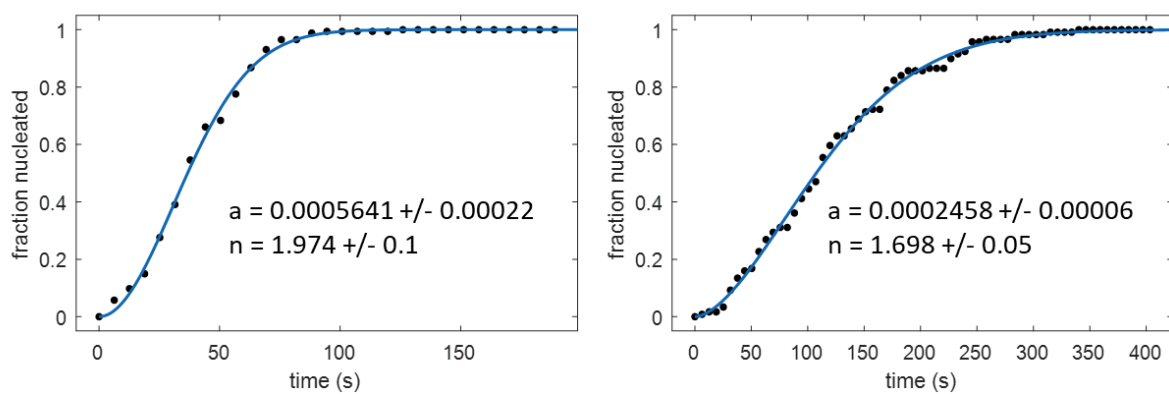

**Fig. S12. Nucleation events versus time and Avrami fits.**

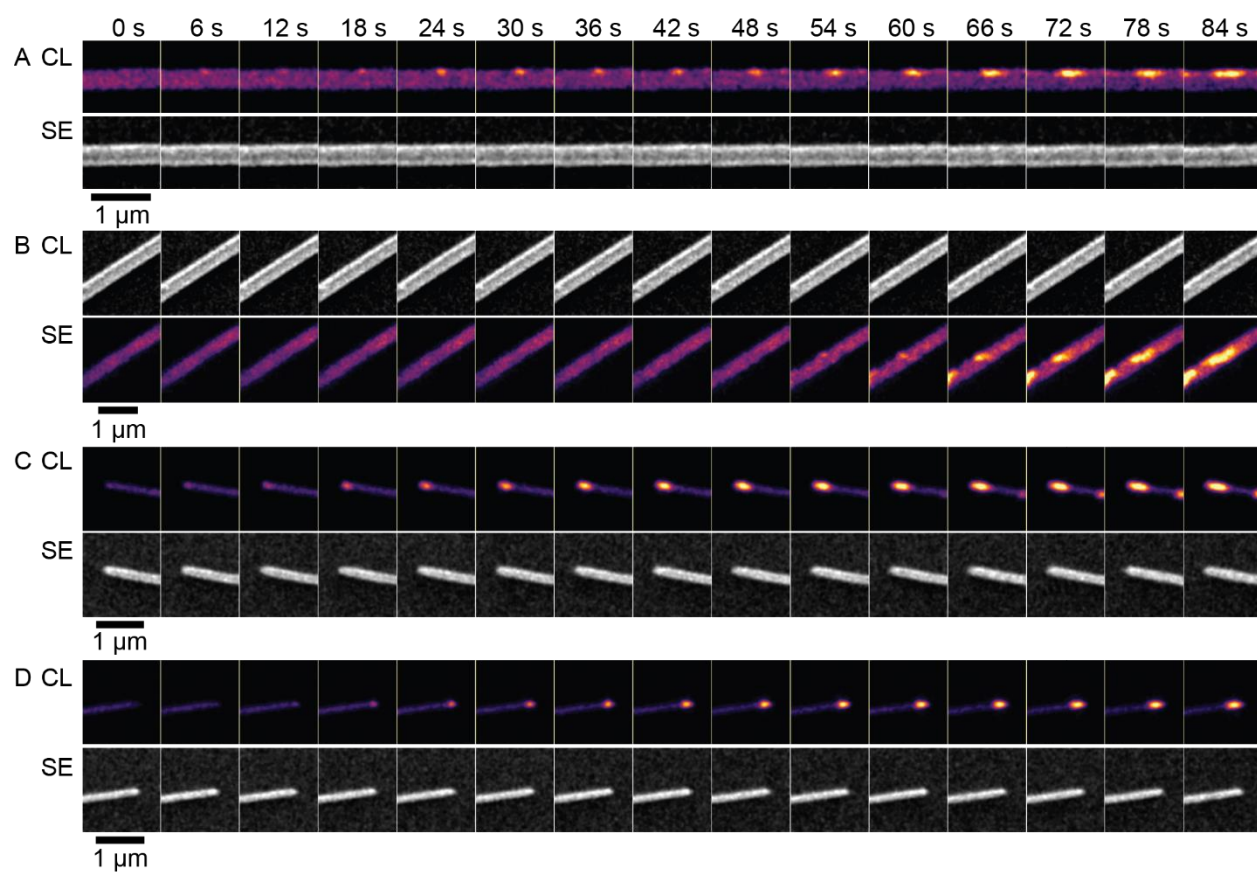

**Fig. S13. Additional single nucleation events at nanowire ends and sides.** CL and SE time series of nucleation events at (A-B) nanowire ends and (C-D) nanowire sides.

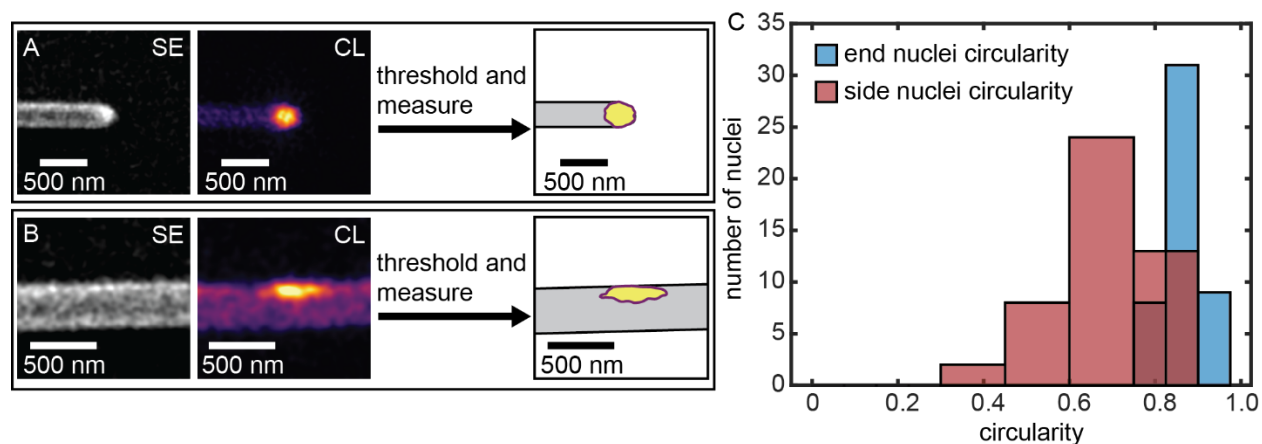

**Fig. S14. Circularity analysis of nuclei.** Example of circularity measurements for (A) end and (B) side nuclei. An intensity threshold above the background CL of the LT-CsPbIBr<sub>2</sub> nanowire is applied and the area and perimeter of each nucleus is used to determine the circularity parameter. (C) Histograms of the circularity of nuclei for end and side nucleation events. The average circularity for end nuclei is 0.86 (standard deviation is 0.046, N = 48) and the average circularity for side nuclei is 0.67 (standard deviation is 0.12, N = 48).

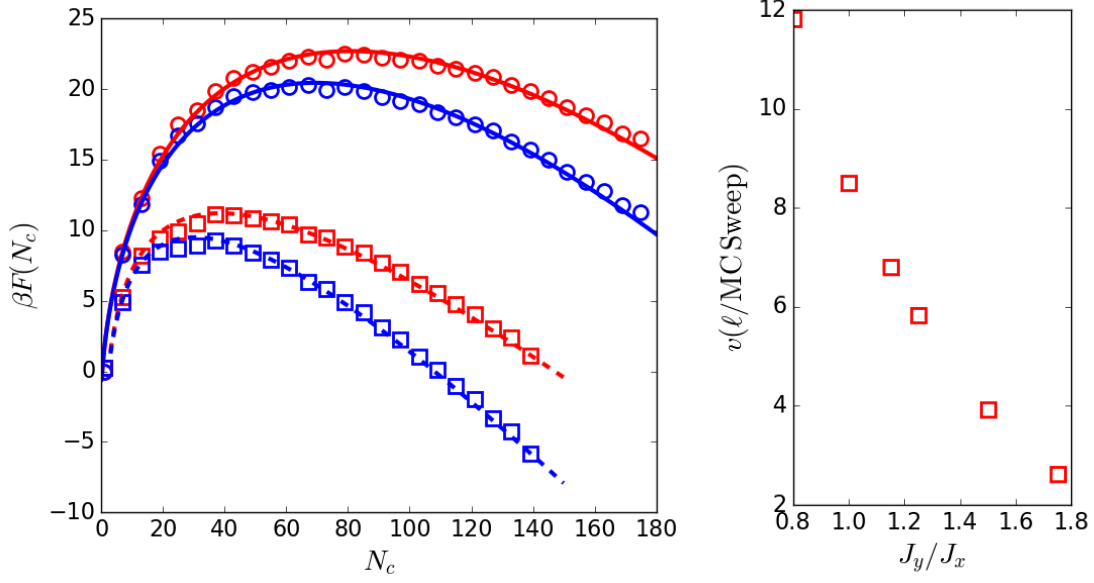

**Fig. S15. Nucleation and growth for the Ising model.** (A) Free energy as a function of cluster size for side and end growth in blue and red respectively. The circles are for  $J_y/J_x = 1.5$  and the squares are for  $J_y/J_x = 1$ . (B) Phase growth velocity along the direction of the long axis as a function of  $J_x/J_y$  in units of lattice length and Monte Carlo sweeps.

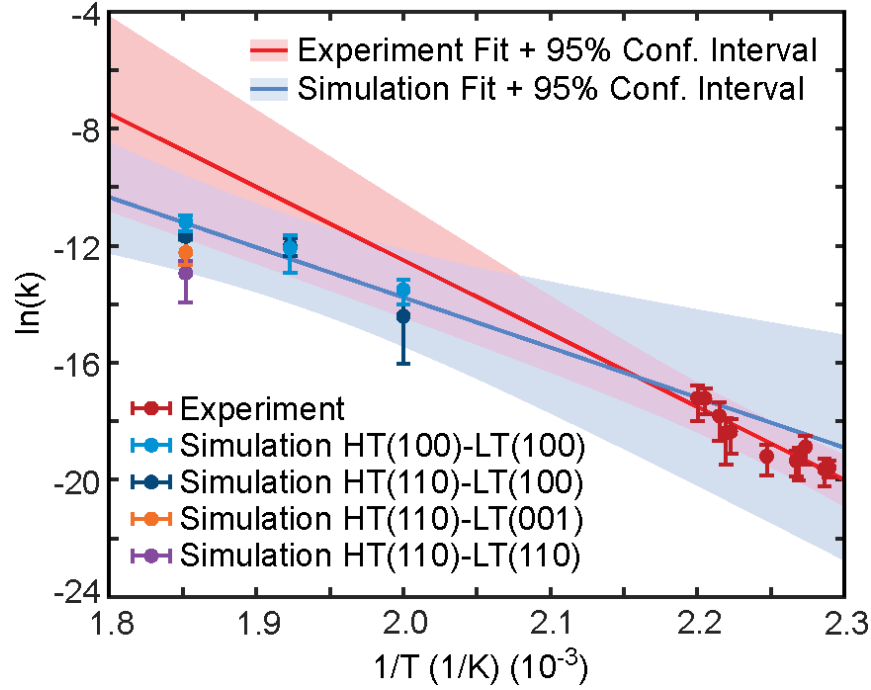

**Fig. S6. Arrhenius plot of experimental data and simulation data.** A reproduction of Figure 2B of the main text with additional information. In addition to the experimental (red) and simulation (light and dark blue) data and respective fits and 95% fit confidence intervals, the orange and purple data points represent growth of the  $\langle 110 \rangle$  HT-CsPbBr<sub>3</sub> plane *parallel* to the wire axis in contact with the  $\langle 010 \rangle$  and  $\langle 001 \rangle$  planes of the LT-CsPbBr<sub>3</sub> phase, respectively. These data are not included in the fit, as they represent slower growth in a direction orthogonal to the wire axis of primary relevance to the discussion of Figure 3 in the main text.

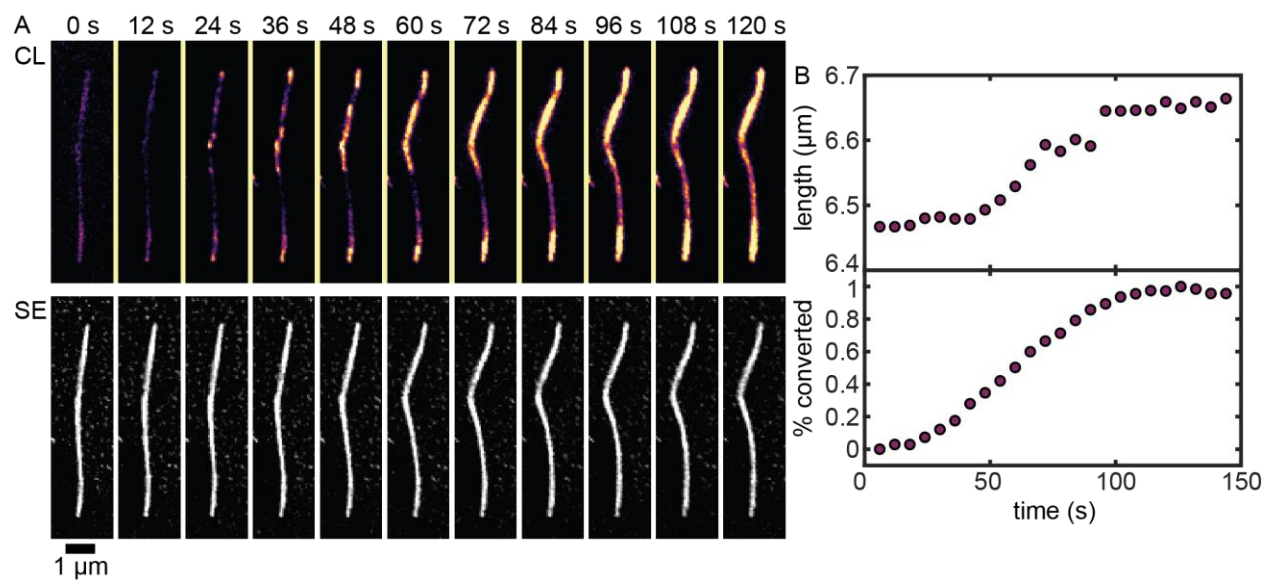

**Fig. S7. Nanowire bending and expansion upon phase transition.** (A) CL and SE time series showing a nanowire bending during the phase transition. (B) The length of the wire (above) is correlated to the percent of the nanowire converted to the HT-CsPbIBr<sub>2</sub> phase.

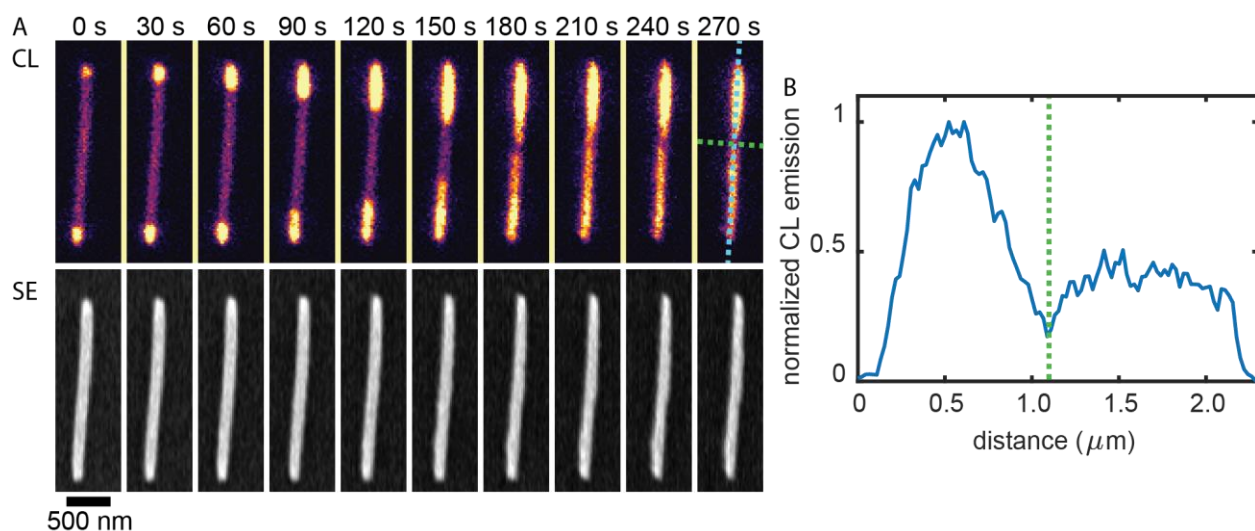

**Fig. S8. SE and CL images of nanowire phase boundaries where two fronts meet.** (A) SE and CL images of a time series showing phase propagation. (B) Cross-section of the CL image at 270 s (across the blue dotted line in A). The green dotted line signifies where the two phase fronts meet in the middle of the nanowire.

## Supplementary Tables

**Table S1.** Force field parameters.

|    | $\varepsilon$ (eV) | $\sigma$ (Å) | $q$ (e) |
|----|--------------------|--------------|---------|
| Cs | 0.5784             | 2.927        | 0.86    |
| Pb | 0.01071            | 2.524        | 1.03    |
| Br | 0.01023            | 4.129        | -0.63   |

**Table S2.** Physical properties of five structures of CsPbBr<sub>3</sub> calculated with our force field, DFT-PBEsol, DFT-PBE, and DFT-SCAN, together with available experimental results. Lattice parameters  $a$ ,  $b$ , and  $c$  are given in units of Å; elastic constants  $c_{ij}$  in units of GPa; bulk modulus  $B$  in GPa; and energy differences  $\Delta E$  with respect to the ground state orthorhombic perovskite structure in meV/f.u.. Values in bold face were used for fitting.

|                                                         | Force field | DFT          |           |       | Experiment    |
|---------------------------------------------------------|-------------|--------------|-----------|-------|---------------|
|                                                         |             | PBEsol       | PBE       | SCAN  |               |
| Cubic perovskite structure (space group #221)           |             |              |           |       |               |
| $a$                                                     | 5.79        | <b>5.76</b>  | 5.89      | 5.874 | 5.874 (600 K) |
| $c_{11}$                                                | 51.4        | <b>51.9</b>  | -         | -     | -             |
| $c_{44}$                                                | 6.6         | <b>6.4</b>   | -         | -     | -             |
| $c_{66}$                                                | 6.6         | <b>4.1</b>   | -         | -     | -             |
| $B$                                                     | 21.6        | <b>21.6</b>  | -         | -     | -             |
| $\Delta E$                                              | 84          | 108          | <b>84</b> | 90    | -             |
| Tetragonal-a perovskite structure (space group #127)    |             |              |           |       |               |
| $a$                                                     | 8.07        | <b>8.12</b>  | 8.32      | 8.19  | -             |
| $c$                                                     | 5.94        | <b>5.96</b>  | 6.08      | 6.00  | -             |
| $\Delta E$                                              | 23          | -30          | <b>24</b> | 23    | -             |
| Tetragonal-b perovskite structure (space group #140)    |             |              |           |       |               |
| $a$                                                     | 8.07        | <b>8.12</b>  | 8.33      | 8.18  | -             |
| $c$                                                     | 11.89       | <b>11.92</b> | 12.16     | 12.01 | -             |
| $\Delta E$                                              | 23          | -28          | <b>23</b> | 21    | -             |
| Orthorhombic perovskite structure (space group #62)     |             |              |           |       |               |
| $a$                                                     | 8.43        | <b>8.39</b>  | 8.53      | 8.43  | 8.244         |
| $b$                                                     | 11.69       | <b>11.66</b> | 11.91     | 11.76 | 11.735        |
| $c$                                                     | 7.88        | <b>7.97</b>  | 8.26      | 8.07  | 8.198         |
| Orthorhombic non-perovskite structure (space group #62) |             |              |           |       |               |
| $a$                                                     | 9.74        | <b>9.69</b>  | 10.09     | 9.79  | 9.72          |
| $b$                                                     | 4.63        | <b>4.55</b>  | 4.66      | 4.58  | 4.6           |
| $c$                                                     | 16.62       | <b>16.69</b> | 17.21     | 16.85 | 16.81         |
| $\Delta E$                                              | 10          | -12          | <b>10</b> | -29   | -             |

### **Captions for Movies**

**Movie S1.** Large field-of-view SE and CL movies of the LT-CsPbIBr<sub>2</sub> to HT-CsPbIBr<sub>2</sub> phase transition.

**Movie S2.** Molecular dynamics simulation of the propagating phase front

**Movie S3.** SE and CL movies of nucleation at a CsPbIBr<sub>2</sub> nanowire end

**Movie S4.** SE and CL movies of nucleation at a CsPbIBr<sub>2</sub> nanowire side

## References

1. J. Lin *et al.*, Thermochromic halide perovskite solar cells. *Nature Materials*. **17**, 261 (2018).
2. Y. Wang *et al.*, Elucidation of the elusive structure and formula of the active pharmaceutical ingredient bismuth subgallate by continuous rotation electron diffraction. *Chem. Commun.* **53**, 7018–7021 (2017).
3. W. Kabsch, XDS. *Acta Cryst D*. **66**, 125–132 (2010).
4. W. Wan, J. Sun, J. Su, S. Hovmöller, X. Zou, Three-dimensional rotation electron diffraction: software RED for automated data collection and data processing. *J Appl Cryst.* **46**, 1863–1873 (2013).
5. D. B. Durham, D. F. Ogletree, E. S. Barnard, Scanning Auger spectromicroscopy using the ScopeFoundry software platform. *Surface and Interface Analysis*. **50**, 1174–1179 (2018).
6. M. Lai *et al.*, Intrinsic anion diffusivity in lead halide perovskites is facilitated by a soft lattice. *PNAS*. **115**, 11929–11934 (2018).
7. E. Rabani, An interatomic pair potential for cadmium selenide. *J. Chem. Phys.* **116**, 258–262 (2001).
8. *Atoms in Molecules: A Quantum Theory* (Oxford University Press, Oxford, New York, 1994), *International Series of Monographs on Chemistry*.
9. G. Kresse, J. Furthmüller, Efficiency of ab-initio total energy calculations for metals and semiconductors using a plane-wave basis set. *Computational Materials Science*. **6**, 15–50 (1996).
10. P. E. Blöchl, Projector augmented-wave method. *Phys. Rev. B*. **50**, 17953–17979 (1994).
11. J. P. Perdew, K. Burke, M. Ernzerhof, Generalized Gradient Approximation Made Simple. *Phys. Rev. Lett.* **77**, 3865–3868 (1996).
12. J. P. Perdew *et al.*, Restoring the Density-Gradient Expansion for Exchange in Solids and Surfaces. *Phys. Rev. Lett.* **100**, 136406 (2008).
13. J. Sun, A. Ruzsinszky, J. P. Perdew, Strongly Constrained and Appropriately Normed Semilocal Density Functional. *Phys. Rev. Lett.* **115**, 036402 (2015).
14. Y. Rakita *et al.*, Low-Temperature Solution-Grown CsPbBr<sub>3</sub> Single Crystals and Their Characterization. *Crystal Growth & Design*. **16**, 5717–5725 (2016).
15. null Dodson, Development of a many-body Tersoff-type potential for silicon. *Phys. Rev., B Condens. Matter*. **35**, 2795–2798 (1987).

16. E. Iype, M. Hütter, A. P. J. Jansen, S. V. Nedea, C. C. M. Rindt, Parameterization of a reactive force field using a Monte Carlo algorithm. *J Comput Chem.* **34**, 1143–1154 (2013).
17. J. D. Gale, A. L. Rohl, The General Utility Lattice Program (GULP). *Molecular Simulation.* **29**, 291–341 (2003).
18. S. Plimpton, Fast Parallel Algorithms for Short-Range Molecular Dynamics. *Journal of Computational Physics.* **117**, 1–19 (1995).
19. D. Chandler, *Introduction to Modern Statistical Mechanics* (Oxford University Press, New York, 1 edition., 1987).
20. A. C. Pan, D. Chandler, Dynamics of Nucleation in the Ising Model. *J. Phys. Chem. B.* **108**, 19681–19686 (2004).
